# Supplementary material for: Polarized photoluminescence clocks ultrafast pseudospin relaxation in graphene
Source: arXiv:1702.00962 ancillary file (2017-02-03)
Supplement: Supplementary file 1 [file supplemental_material.pdf]

# Supplemental Material: Polarized photoluminescence clocks ultrafast pseudospin relaxation in graphene

Thomas Danz,[1,2] Andreas Neff,[1,2,*] John H. Gaida,[1]
Reiner Bormann,[1] Claus Ropers,[1] and Sascha Schäfer[1,†]

[1] *4th Physical Institute – Solids and Nanostructures,*
*University of Göttingen, Göttingen, Germany*
[2] *These authors contributed equally to this work.*

(Dated: January 24, 2017)

## I. EXPERIMENTAL DETAILS

### A. Experimental setup

The experimental setup is schematically depicted in Fig. 1. Graphene samples are excited under ambient conditions by 18 fs ultrashort laser pulses at a central wavelength of 800 nm generated by a mode-locked Ti:sapphire oscillator at a repetition rate of 80 MHz. After passing an attenuator (half-wave plate and polarizer) and a low-pass filter in order to remove residual green light, the pump beam is focused onto the sample at normal incidence ($43 \pm 10\,\mu$m FWHM pump spot diameter), and the emerging PL is aspherically and achromatically collected in a transmission geometry using a low-scatter off-axis parabolic mirror (NA $\approx 0.45$). After blocking the pump laser light using a high-pass filter, the blue-shifted PL emission is detected in a polarization-resolved and time-integrated manner by a liquid nitrogen-cooled charge-coupled device (CCD) attached to a grating spectrometer (typical integration time of 10 s). For determining the PL spectral shape, we consider the wavelength-dependent sensitivity of the spectrometer and CCD detector as specified by the manufacturer. The relative spectral sensitivity for horizontally and vertically polarized light was determined using the continuous spectrum of a xenon arc lamp filtered by a broadband

* Present address: Leibniz Institute of Surface Modification, Leipzig, Germany
† schaefer@ph4.physik.uni-goettingen.de

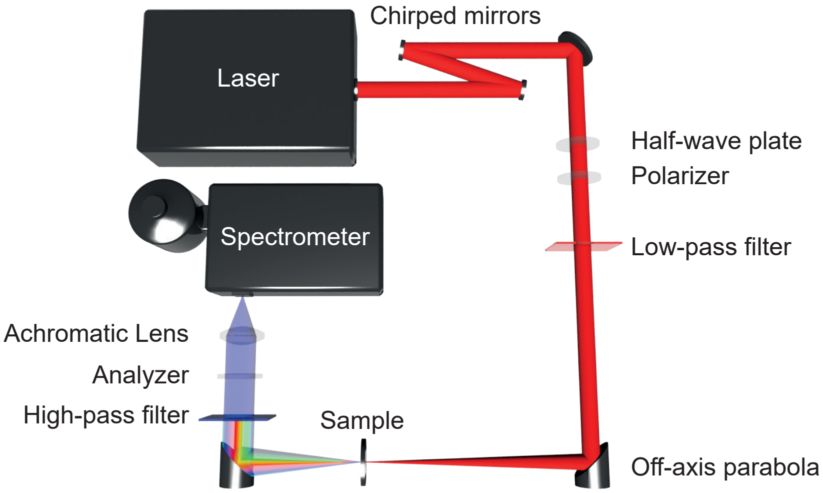


FIG. 1. Schematic view of the experimental setup.

polarizer. We estimate a wavelength-dependent total PL detection efficiency of about 0.6 % to 2.3 %, which includes contributions from the collection optics (7 %), the high-pass filter (14 % to 83 %), the diffraction efficiency at the spectrometer grating (30 % to 82 %), and the detection quantum efficiency of the CCD detector (48 % to 78 %).

### B. Sample preparation

Single-layer graphene was grown by chemical vapor deposition (CVD) on tempered polycrystalline copper foils [1] (for growth parameters see supplementary materials of Ref. 2). The graphene layer on one side of the copper foil was transferred onto $\alpha$-$Al_2O_3(0\,0\,0\,1)$ substrates (C-plane sapphire) by first spin-coating a protective poly(methyl methacrylate) (PMMA) layer on top of graphene, removing the back-side graphene by reactive-ion etching, and dissolving copper in a 0.3 M solution of ammonium persulfate [3]. After rinsing the floating graphene using deionized water, we transferred it onto the sapphire substrate, and dissolved the PMMA protection layer by rinsing the dried sample with acetone, isopropanol and deionized water. Graphene on sapphire as fabricated here is expected to exhibit a slight p-doping with a Fermi energy of about 100 meV below the energy at the Dirac point [4]. Using resonant Raman spectroscopy, we verified that the sample has monolayer thickness [1, 5, 6]. PL scans of the sample surface served to monitor the homogeneity of the prepared graphene samples (see Fig. 2).

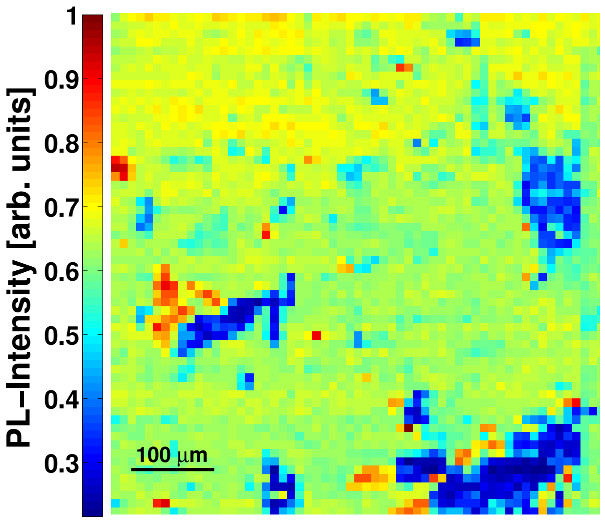


FIG. 2. Spectrally integrated PL scan of an exemplary graphene sample as prepared using the described procedure. The homogenous PL signal over large areas indicates a good sample quality. The slightly larger signal in the upper part of the scan is most likely due to a minor tilt of the sample.

## II. BOLTZMANN RATE EQUATIONS

In the following, we outline our numerical approach for describing carrier dynamics in graphene based on Boltzmann rate equations [7]. As introduced in the main text, we approximate graphene's carrier distribution by a superposition of a parallel and a perpendicular component, following the symmetry of the carrier-field coupling matrix elements [8]. The general expression of the carrier distribution is given by

$$f_c(\varepsilon, \varphi, t) = f_{c,\|}(\varepsilon, t)\, \sin^2 \varphi + f_{c,\perp}(\varepsilon, t)\, \cos^2 \varphi. \qquad (1)$$

Both components of the overall carrier occupation contain half of the density of states $D_{\|}(\varepsilon) = D_{\perp}(\varepsilon) = D(\varepsilon)/2 = |\varepsilon|/\pi\hbar^2 v_F^2$, where $v_F \approx 1 \times 10^6\,\mathrm{m/s}$ is the Fermi velocity [9]. Graphene doping by the sapphire substrate is neglected, so that the Fermi energy $\varepsilon_F$ is zero. Prior to optical excitation, the system is in an isotropic equilibrium state at a temperature of 300 K.

## A. Photon absorption

The carrier-field coupling matrix element of graphene has been derived in earlier works on the basis of a tight-binding (TB) approximation for the dispersion relation $\varepsilon(\boldsymbol{k})$ [8, 10, 11]. The matrix element $\boldsymbol{M}^{vc}(\boldsymbol{k})$ describes the probability of an electron of momentum $\boldsymbol{k}$ being promoted from the valence band $v$ into the conduction band $c$ due to interaction with an external electromagnetic field. Since all relevant physical processes involved in sample excitation and relaxation take place in the low-energy optical regime, the full TB dispersion relation may be approximated by a linear dispersion around the $K$ (and $K'$) points of the first Brillouin zone with $\boldsymbol{q} = \boldsymbol{k} - \boldsymbol{K}$ (and $\boldsymbol{q} = \boldsymbol{k} - \boldsymbol{K'}$ respectively), i. e. $\varepsilon(\boldsymbol{q}) = \pm\hbar v_F|\boldsymbol{q}|$. In this approximation and in the vicinity of the $K$ and $K'$ points, the carrier-field coupling matrix element between electron and hole states with momentum $\boldsymbol{q}$ is a function of the angle $\varphi$ between the direction of carrier momentum in the Dirac cone and the $\hat{\boldsymbol{q}}_{\boldsymbol{x}}$ axis. Thus, we can write

$$\boldsymbol{M}^{vc}(\varphi) = \begin{pmatrix} M_x^{vc} \\ M_y^{vc} \end{pmatrix} \propto \begin{pmatrix} \sin\varphi \\ \cos\varphi \end{pmatrix} \tag{2}$$

with $\tan\varphi = q_y/q_x$. The matrix element obeys the relation $|\boldsymbol{M}^{vc}(\varphi)|^2 = \text{const.}$, as expected according to the isotropic character of low-energy excitations in graphene.

After absorption of a laser pulse with polarization unit vector $\boldsymbol{P} = \hat{\boldsymbol{x}}$, the angular dependency of the resulting anisotropic electron distribution is given by

$$f_c(\varepsilon,\varphi) \propto |\boldsymbol{P}\cdot\boldsymbol{M}^{vc}|^2 = \sin^2\varphi. \tag{3}$$

Accordingly, sample excitation with $\hat{\boldsymbol{x}}$ polarized laser pulses leads to a non-equilibrium electron occupation in the conduction band in $\hat{\boldsymbol{q}}_{\boldsymbol{y}}$ direction, while no change in occupation is observed in the $\hat{\boldsymbol{q}}_{\boldsymbol{x}}$ direction (and vice versa for $\boldsymbol{P} = \hat{\boldsymbol{y}}$). Adopting the two-component carrier distribution introduced in Eq. 1, optical excitation initially only populates the component $f_{c,\parallel}$ of the carrier distribution. The change of the electron distribution due to laser pulse absorption at normal incidence is given by Ref. 12:

$$\dot{f}^{abs}_{c,\parallel}(\varepsilon) = 2\pi\alpha\, n(2\varepsilon,t)\frac{f_{v,\parallel}(-\varepsilon,t) - f_{c,\parallel}(\varepsilon,t)}{D_\parallel(\varepsilon)}. \tag{4}$$

Here, $\alpha$ is the fine-structure constant, and $n$ the incident photon flux. Absorption of a laser pulse leads to a non-equilibrium distribution of electrons and holes around half the pump photon energy.

### B. Photon emission

Since the matrix elements for photon absorption and emission are equal, i. e. $\boldsymbol{M}^{vc}(\varphi) = \boldsymbol{M}^{cv}(\varphi)$, the formula for the polarization-resolved PL intensities [12, 13] can be written as:

$$\widetilde{I}_{\parallel}(2\varepsilon, t) \propto \int_0^{2\pi} |M_x^{vc}(\varphi)|^2 \, f_c(\varepsilon, \varphi, t) \, [1 - f_v(-\varepsilon, \varphi, t)] \, \mathrm{d}\varphi \,, \tag{5}$$

$$\widetilde{I}_{\perp}(2\varepsilon, t) \propto \int_0^{2\pi} \left|M_y^{vc}(\varphi)\right|^2 f_c(\varepsilon, \varphi, t) \, [1 - f_v(-\varepsilon, \varphi, t)] \, \mathrm{d}\varphi \,. \tag{6}$$

Integrating both equations and considering $f_v(-\varepsilon, \varphi, t) = 1 - f_c(\varepsilon, \varphi, t)$, we find:

$$\widetilde{I}_{\parallel}(2\varepsilon, t) \propto 5 f_{c,\parallel}^2(\varepsilon, t) + 2 f_{c,\parallel}(\varepsilon, t) \, f_{c,\perp}(\varepsilon, t) + f_{c,\perp}^2(\varepsilon, t), \tag{7}$$

$$\widetilde{I}_{\perp}(2\varepsilon, t) \propto 5 f_{c,\perp}^2(\varepsilon, t) + 2 f_{c,\parallel}(\varepsilon, t) \, f_{c,\perp}(\varepsilon, t) + f_{c,\parallel}^2(\varepsilon, t). \tag{8}$$

Therefore, even without taking any relaxation processes into account, the initial $\sin^2\varphi$-shaped carrier distribution radiates off by electron-hole recombination not only with $\hat{\boldsymbol{x}}$ polarization, but to some extent also with $\hat{\boldsymbol{y}}$ polarization. Therefore, the transient polarization ratio, defined as

$$\widetilde{R}(2\varepsilon, t) = \frac{\widetilde{I}_{\parallel}(2\varepsilon, t)}{\widetilde{I}_{\perp}(2\varepsilon, t)}, \tag{9}$$

reaches its highest value of 5 directly after carrier excitation. Any subsequent relaxation process transfers occupation to the perpendicular carrier distribution $f_{c,\perp}$, further reducing the transient polarization ratio. Thus, the maximum value of $\widetilde{R} = 5$ also gives a physical upper bound for the experimentally measured time-integrated polarization ratio introduced in the main text:

$$R(2\varepsilon) = \frac{I_{\parallel}(2\varepsilon)}{I_{\perp}(2\varepsilon)} = \frac{\int_0^\infty \widetilde{I}_{\parallel}(2\varepsilon, t) \, \mathrm{d}t}{\int_0^\infty \widetilde{I}_{\perp}(2\varepsilon, t) \, \mathrm{d}t}. \tag{10}$$

For obtaining an absolute scale for the emitted PL flux (cf. Fig. 2a of the main text), we infer the angle-averaged photon emission flux from Ref. 12, resulting in

$$\dot{p}(2\varepsilon) = \frac{4\alpha}{3\epsilon_r} \frac{v_F^2}{c^2} \frac{\varepsilon}{\hbar} f_c^{\mathrm{iso}}(\varepsilon, t) \left[1 - f_v^{\mathrm{iso}}(-\varepsilon, t)\right] D(\varepsilon) \tag{11}$$

for the case of an isotropic carrier distribution. For $\epsilon_r$ we consider the average relative permittivity of the surrounding media, and $f_c^{\mathrm{iso}}$ is approximated as $f_c^{\mathrm{iso}}(\varepsilon, t) \approx [f_{c,\parallel}(\varepsilon, t) + f_{c,\perp}(\varepsilon, t)]/2$.

The transient photon flux $\dot{p}_{\|}(2\varepsilon)$ and $\dot{p}_{\perp}(2\varepsilon)$ detected after linear polarizers with parallel or perpendicular orientation (relative to the optical pulse), respectively, is then given by:

$$\dot{p}_{\|}(2\varepsilon) = \frac{\dot{p}(2\varepsilon)}{1+\widetilde{R}(2\varepsilon,t)^{-1}}, \tag{12}$$

$$\dot{p}_{\perp}(2\varepsilon) = \frac{\dot{p}(2\varepsilon)}{1+\widetilde{R}(2\varepsilon,t)}. \tag{13}$$

### C. Carrier-carrier scattering

The carrier-carrier scattering rate is given by Fermi's golden rule [14]. For each component of the carrier distribution separately, we consider scattering processes within an isotropic distribution, such that carrier-carrier scattering can be treated in an angle-integrated manner. The possible scattering events, excluding Auger processes, are CCCC, VVVV, CVCV and CCVV, for which the second and third letter denote the band of the incident electrons and the first and fourth letter the bands of the electrons after scattering [15]. Thus, the scattering integral has to be solved for all of these processes. For example for CCCC processes, the change of the electron distribution is given by [16]

$$\dot{f}_c^{CCCC}(\boldsymbol{k}_1) = R_1^{CCCC}(\boldsymbol{k}_1) + R_2^{CCCC}(\boldsymbol{k}_1) \tag{14}$$

with

$$\begin{aligned} R_1^{CCCC}(\boldsymbol{k}_1) = \frac{2\pi}{\hbar^2 v_F} \int \frac{\mathrm{d}\boldsymbol{k}_2}{(2\pi)^2} \int \frac{\mathrm{d}\boldsymbol{k}_1'}{(2\pi)^2} V_{c\ \boldsymbol{k}_1, c\ \boldsymbol{k}_2}^{c\ \boldsymbol{k}_1', c\ \boldsymbol{k}_2'} \\ \cdot f_c(|\boldsymbol{k}_1|) f_c(|\boldsymbol{k}_2|) \left[1 - f_c(|\boldsymbol{k}_1'|)\right] \left[1 - f_c(|\boldsymbol{k}_2'|)\right] \\ \cdot \delta\left(|\boldsymbol{k}_1| + |\boldsymbol{k}_2| - |\boldsymbol{k}_1'| - |\boldsymbol{k}_2'|\right), \end{aligned} \tag{15}$$

$$\begin{aligned} R_2^{CCCC}(\boldsymbol{k}_1) = -\frac{2\pi}{\hbar^2 v_F} \int \frac{\mathrm{d}\boldsymbol{k}_2}{(2\pi)^2} \int \frac{\mathrm{d}\boldsymbol{k}_1'}{(2\pi)^2} V_{c\ \boldsymbol{k}_1', c\ \boldsymbol{k}_2'}^{c\ \boldsymbol{k}_1, c\ \boldsymbol{k}_2} \\ \cdot f_c(|\boldsymbol{k}_1'|) f_c(|\boldsymbol{k}_2'|) \left[1 - f_c(|\boldsymbol{k}_1|)\right] \left[1 - f_c(|\boldsymbol{k}_2|)\right] \\ \cdot \delta\left(|\boldsymbol{k}_1| + |\boldsymbol{k}_2| - |\boldsymbol{k}_1'| - |\boldsymbol{k}_2'|\right). \end{aligned} \tag{16}$$

$\boldsymbol{k}_1$ and $\boldsymbol{k}_2$ are the electron wave vectors before scattering, and $\boldsymbol{k}_1'$ and $\boldsymbol{k}_2' = \boldsymbol{k}_1 + \boldsymbol{k}_2 - \boldsymbol{k}_1'$ the wave vectors after scattering. The delta function ensures energy conservation. The terms $R_{1,2}^{CCCC}$ correspond to scattering processes increasing and decreasing the occupation of carrier momentum $\boldsymbol{k}_1$, respectively. The matrix element for electron-electron scattering in graphene

can be written as [17, 18]

$$V_{l_1,l_2}^{l'_1,l'_2} = \frac{1}{4}\left(|V_d|^2 + |V_e|^2 - |V_d - V_e|^2\right). \tag{17}$$

The combined indices $\boldsymbol{l}$ contain the band indices and the electron wave vectors. $V_d$ is the matrix element for direct scattering, and $V_e$ for exchange scattering. Making use of the delta function in Eqns. 15 and 16 allows to reduce the four-dimensional integrals to three dimensions, which are then numerically evaluated by Monte Carlo integration [16].

The scattering integral for Auger processes is analogous to Eqns. 15 and 16. However, it was shown that Auger scattering can only take place with the involved carrier momenta aligned in a collinear fashion [18, 19]. Thereby, we are able to reduce the integrals to two dimensions by analytical angular integration [18]. The remaining integrals were computed numerically.

### D. Carrier-phonon Scattering

We explicitly consider angle-integrated carrier-phonon scattering with the highest optical phonon branches, which were previously shown to dominate the energy loss of the carrier system at carrier temperatures above 300 K [20–23]. The scattering integral is calculated according to Ref. 21, and a phenomenological decay of the optical phonon distribution with a time constant of 1.2 ps accounts for subsequent phonon-phonon interactions [24].

---


[1] X. Li, W. Cai, J. An, S. Kim, J. Nah, D. Yang, R. Piner, A. Velamakanni, I. Jung, E. Tutuc, S. K. Banerjee, L. Colombo, and R. S. Ruoff, Science **324**, 1312 (2009).

[2] M. Gulde, S. Schweda, G. Storeck, M. Maiti, H. K. Yu, A. M. Wodtke, S. Schäfer, and C. Ropers, Science **345**, 200 (2014).

[3] C. Mattevi, H. Kim, and M. Chhowalla, J. Mater. Chem. **21**, 3324 (2011).

[4] Q. H. Wang, Z. Jin, K. K. Kim, A. J. Hilmer, G. L. C. Paulus, C.-J. Shih, M.-H. Ham, J. D. Sanchez-Yamagishi, K. Watanabe, T. Taniguchi, J. Kong, P. Jarillo-Herrero, and M. S. Strano, Nat. Chem. **4**, 724 (2012).

[5] A. C. Ferrari, J. C. Meyer, V. Scardaci, C. Casiraghi, M. Lazzeri, F. Mauri, S. Piscanec, D. Jiang, K. S. Novoselov, S. Roth, and A. K. Geim, Phys. Rev. Lett. **97**, 187401 (2006).

[6] L. M. Malard, M. A. Pimenta, G. Dresselhaus, and M. S. Dresselhaus, Phys. Rep. **473**, 51 (2009).

[7] J. M. Ziman, *Electrons and Phonons* (Oxford University Press, London, 1960).

[8] E. Malic, T. Winzer, E. Bobkin, and A. Knorr, Phys. Rev. B **84**, 205406 (2011).

[9] A. H. Castro Neto, F. Guinea, N. M. R. Peres, K. S. Novoselov, and A. K. Geim, Rev. Mod. Phys. **81**, 109 (2009).

[10] R. Saito, G. Dresselhaus, and M. S. Dresselhaus, *Physical Properties of Carbon Nanotubes* (Imperial College Press, London, 1998).

[11] A. Grüneis, R. Saito, G. G. Samsonidze, T. Kimura, M. A. Pimenta, A. Jorio, A. G. Souza Filho, G. Dresselhaus, and M. S. Dresselhaus, Phys. Rev. B **67**, 165402 (2003).

[12] M. Mecklenburg, J. Woo, and B. C. Regan, Phys. Rev. B **81**, 245401 (2010).

[13] T. Winzer, R. Ciesielski, M. Handloser, A. Comin, A. Hartschuh, and E. Malic, Nano Lett. **15**, 1141 (2015).

[14] E. Fermi, *Nuclear Physics*, 4th ed. (The University of Chicago Press, Chicago, IL, 1953).

[15] R. Kim, V. Perebeinos, and P. Avouris, Phys. Rev. B **84**, 075449 (2011).

[16] X. Li, E. A. Barry, J. M. Zavada, M. B. Nardelli, and K. W. Kim, Appl. Phys. Lett. **97**, 082101 (2010).

[17] A. Mošková and M. Moško, Phys. Rev. B **49**, 7443 (1994).

[18] F. Rana, Phys. Rev. B **76**, 155431 (2007).

[19] D. Brida, A. Tomadin, C. Manzoni, Y. J. Kim, A. Lombardo, S. Milana, R. R. Nair, K. S. Novoselov, A. C. Ferrari, G. Cerullo, and M. Polini, Nat. Commun. **4**, 1987 (2013).

[20] T. Kampfrath, L. Perfetti, F. Schapper, C. Frischkorn, and M. Wolf, Phys. Rev. Lett. **95**, 187403 (2005).

[21] S. Butscher, F. Milde, M. Hirtschulz, E. Malić, and A. Knorr, Appl. Phys. Lett. **91**, 203103 (2007).

[22] W.-K. Tse and S. Das Sarma, Phys. Rev. B **79**, 235406 (2009).

[23] T. Koyama, Y. Ito, K. Yoshida, M. Tsuji, H. Ago, H. Kishida, and A. Nakamura, ACS Nano **7**, 2335 (2013).

[24] K. Kang, D. Abdula, D. G. Cahill, and M. Shim, Phys. Rev. B **81**, 165405 (2010).
